# Supplementary material for: Is Context Helpful for Chat Translation Evaluation?
Source: arXiv:2403.08314 source file (2024-03-13)
Supplement: Supplementary file 1 [file appendix.tex]

\section{Impact of Length (Category \#2)}

\begin{figure*}[htb!]
\begin{subfigure}{0.25\textwidth}
\centering
  \includegraphics[width=\linewidth]{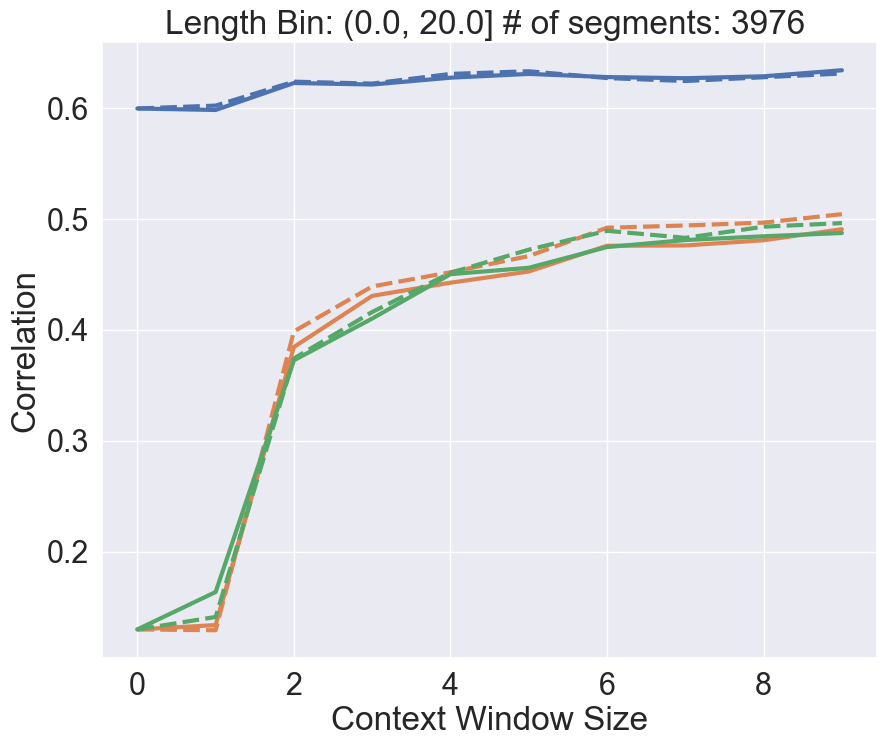}
\end{subfigure}
\begin{subfigure}{0.25\textwidth}
  \centering
  \includegraphics[width=\linewidth]{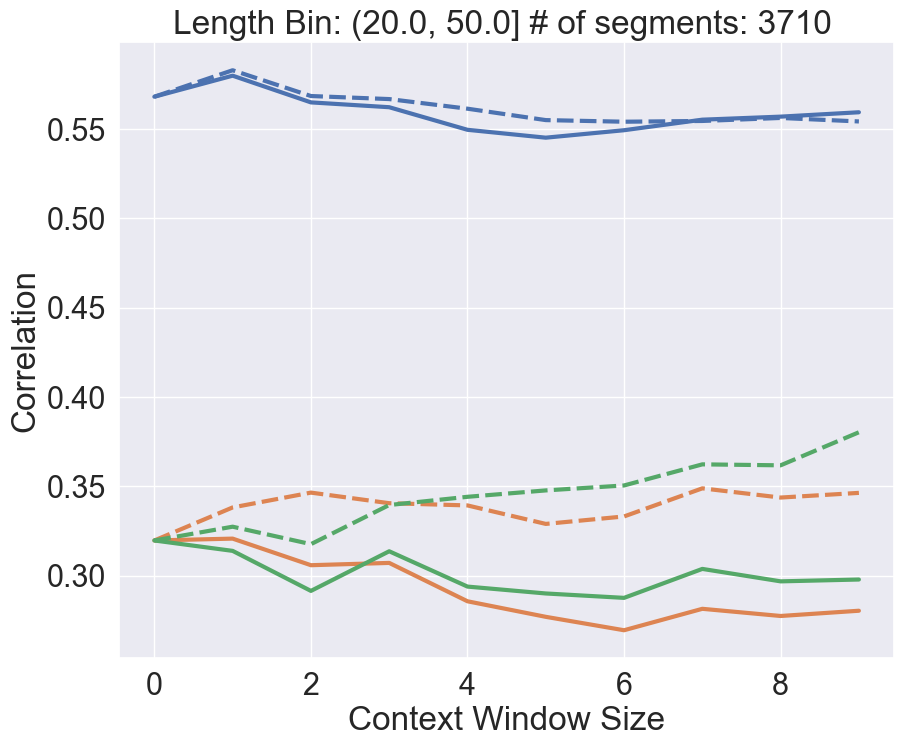}
\end{subfigure}%
\begin{subfigure}{0.25\textwidth}
  \centering
  \includegraphics[width=\linewidth]{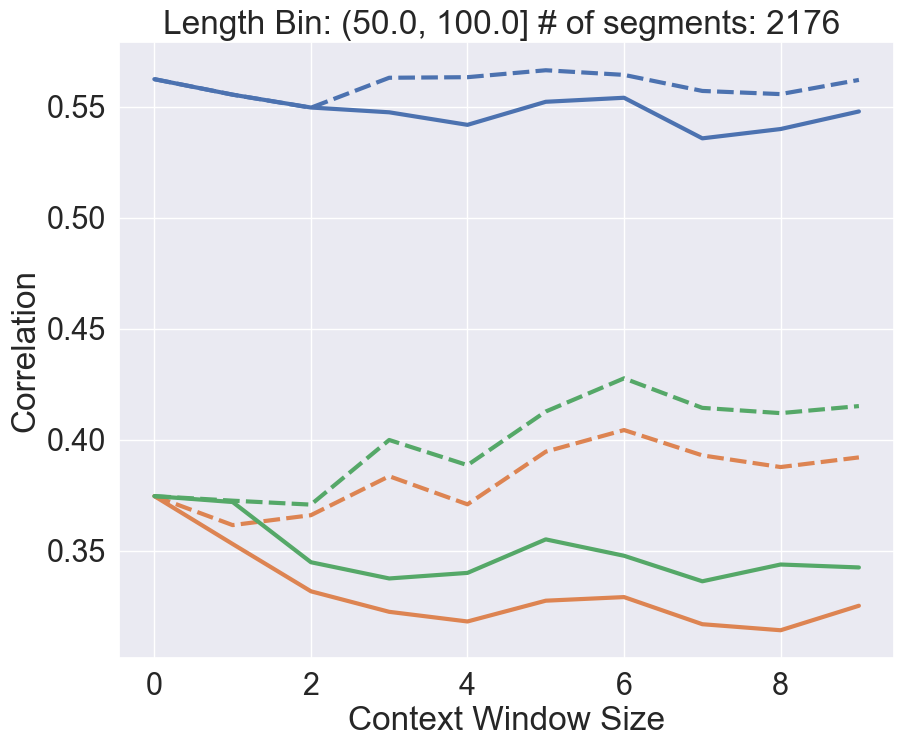}
\end{subfigure}% 
\begin{subfigure}{0.25\textwidth}
  \centering
  \includegraphics[width=\linewidth]{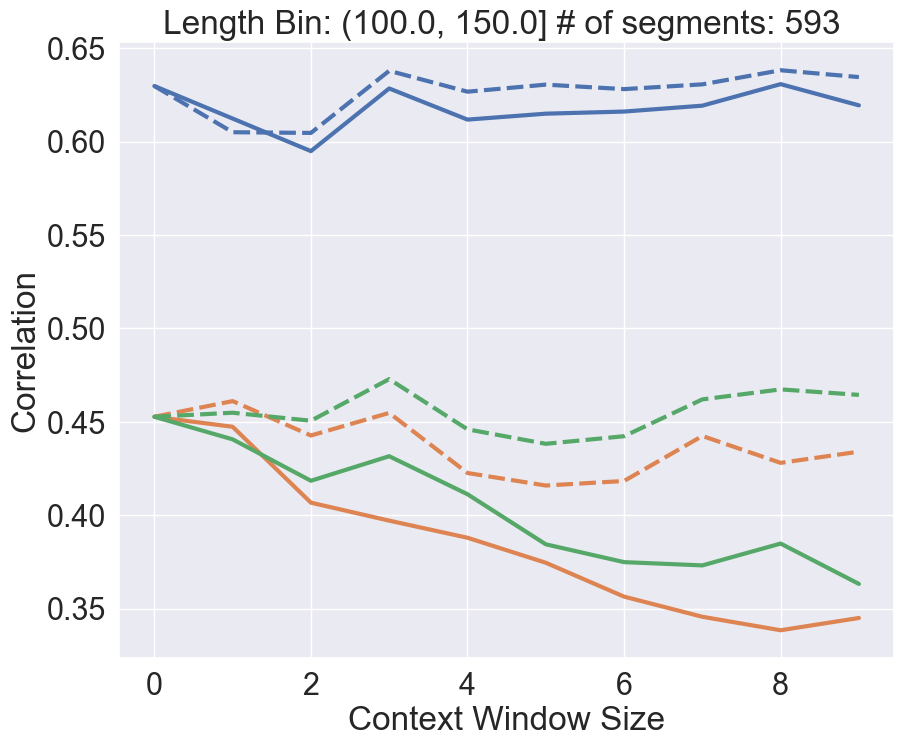}
\end{subfigure}% 
    \caption{Impact of Context on Sequences of different length for Agent Directions.}  \label{fig:contextLengthAgent}
\end{figure*}

\begin{figure*}[htb!]
\begin{subfigure}{0.25\textwidth}
\centering
  \includegraphics[width=\linewidth]{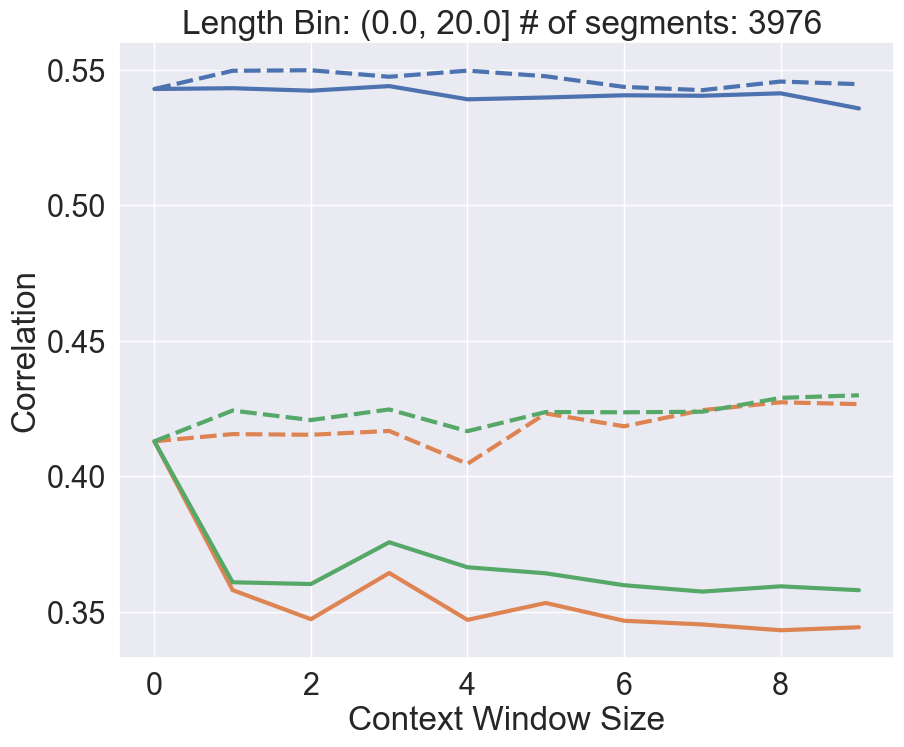}
\end{subfigure}
\begin{subfigure}{0.25\textwidth}
  \centering
  \includegraphics[width=\linewidth]{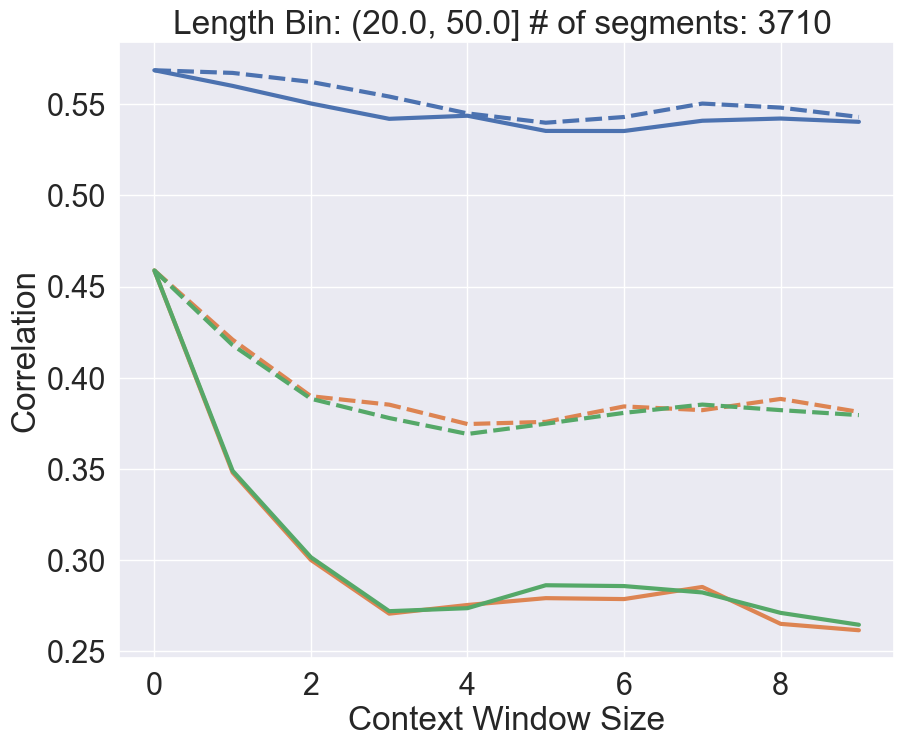}
\end{subfigure}%
\begin{subfigure}{0.25\textwidth}
  \centering
  \includegraphics[width=\linewidth]{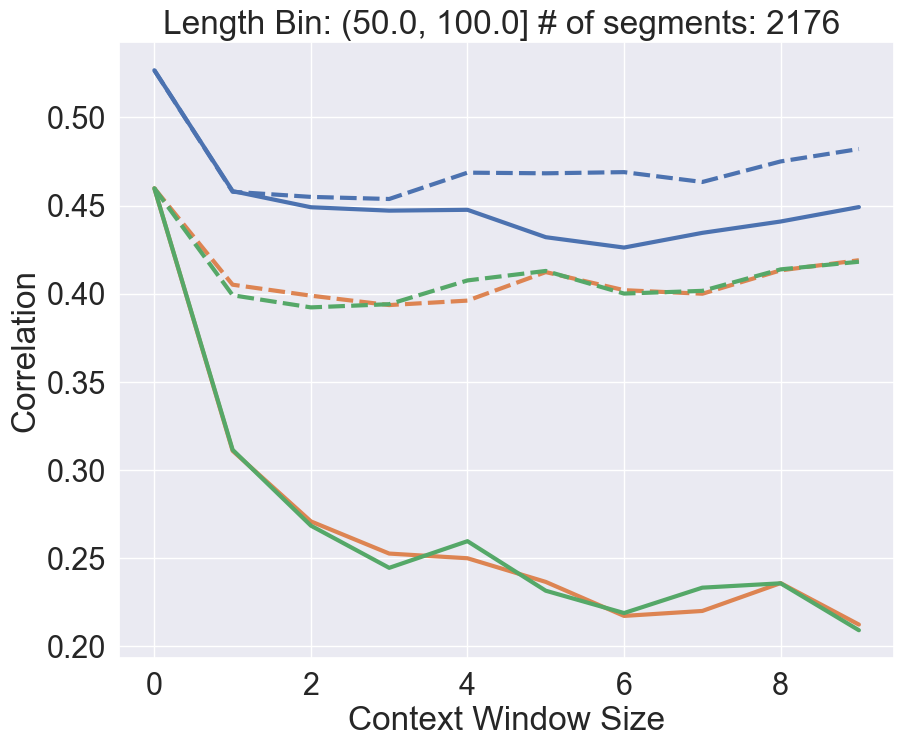}
\end{subfigure}% 
\begin{subfigure}{0.25\textwidth}
  \centering
  \includegraphics[width=\linewidth]{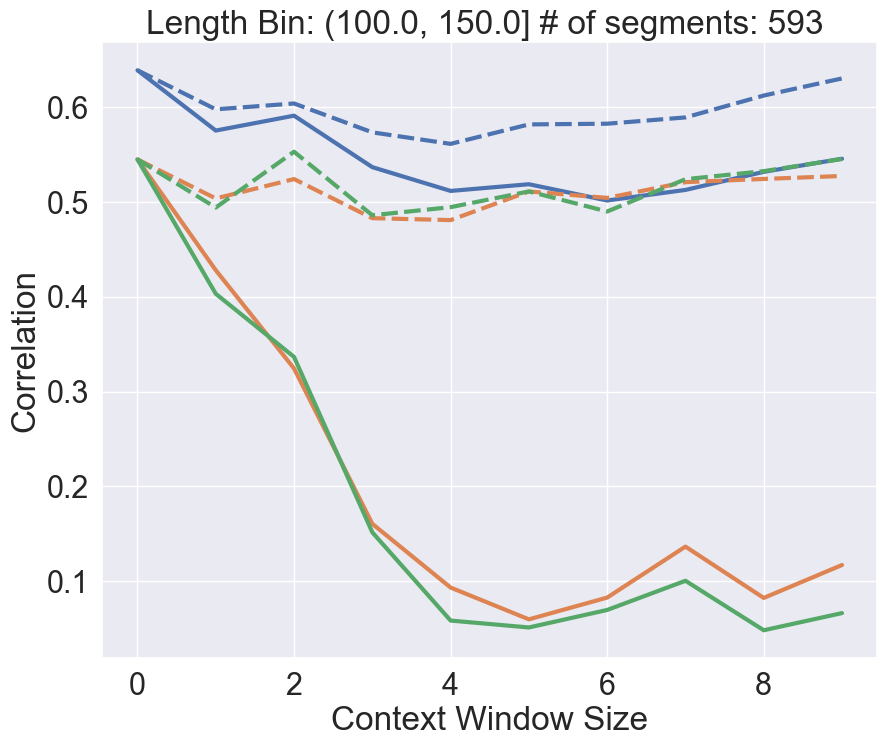}
\end{subfigure}% 
    \caption{Impact of Context on Sequences of different length for Customer Directions.}  \label{fig:contextLengthCustomer}
\end{figure*}
